# Supplementary material for: SurfaceNet+: An End-to-end 3D Neural Network for Very Sparse Multi-view Stereopsis
Source: arXiv:2005.12690 source file (2020-05-26)
Supplement: Supplementary file 1 [file _x_-appendix.tex]

\begin{appendices}
\newpage

%=========================================================================
\section{appendix} \label{appendix}

how the choose the train/val/test set in the DTU dataset

more figures 

\end{appendices}
